# Supplementary material for: Fact-and-Reflection (FaR) Improves Confidence Calibration of Large Language Models
Source: arXiv:2402.17124 source file (2024-09-08)
Supplement: Supplementary file 1 [file appendix.tex]

\subsection{Implementation Details}
We conduct our experiments on 4 GTX 1080 Ti graphics cards with CUDA 11 installed.

We initialize the comparative simplicity measurement model using the BERT-base model with 110M parameters. We pad the input tokens/sentences with BERT start and end symbols (i.e., [CLS] and [SEP]). The size of the hidden states for \textit{FFNN} blocks is 256. During training, we use Mean Squared Error (MSE) loss as the loss function and stochastic gradient descent (SGD) as the optimizer. We initialize all parameters randomly and train all the models with 3 epochs. On average, each epoch takes 20 hours. We use the SemEval 2012 English Lexical Simplification shared task as the intermediate evaluation. We use precision@1 and Pearson correlation to evaluate the models. We tune the hyperparameters with uniform sampling for 10 times and set the learning rate as 5e-5 and the maximum phrase length as 15. The results are presented in the main paper. Other component metrics ($P_{\mathit{simp}}$ and $R_{\mathit{meaning}}$) use pretrained weights from the comparative simplicity measurement model and BERT-base model with 110M parameters. We use the Scikit-learn package \footnote{\url{https://scikit-learn.org/}} to compute logistic regression. All parameters are set as default.

\subsection{Details of finding coefficients}

The details of each way to find adversarial examples are introduced in Table~\ref{tab: noise}. Besides substitution, all methods lead to examples with negative examples. A figurative illustration on the effect of involving these noise types can be found in Figure~\ref{fig:target}, where adequacy and simplicity denote the quality of meaning preservation and comparative simplicity change, respectively.

\begin{table}[t]
\small
    \centering
    \begin{tabular}{p{1.5cm}|p{5.5cm}}
    % \begin{tabular}{c|c|c}
    \toprule
      Noise & Description (label)\\
         \midrule
         Substitution & We use the substitution rules from SimplePPDB or SimplePPDB++ to replace the tokens in the input. (simplifying rule: 1; complicating rule: $-1$; no-difference rule: 0)\\
         \midrule
         Drop & We drop the tokens from the gold reference at a certain probability. ($-1$)\\ 
         \midrule
         Additive & We sample a subsequence from another sentence in the corpus and append it at the end of the original sentence. ($-1$)\\ 
         \midrule
          Shuffling & We shuffle the original sentence to break the original semantics. ($-1$)\\   
         \bottomrule
    \end{tabular}
    \caption{Noise types and their descriptions for adversarial example generation. $1, -1, 0$ denote the process to create good/bad/no-difference simplification, respectively.}
    \label{tab: noise}
    
\end{table}

@misc{bai2022constitutional,
      title={Constitutional AI: Harmlessness from AI Feedback}, 
      author={Yuntao Bai and Saurav Kadavath and Sandipan Kundu and Amanda Askell and Jackson Kernion and Andy Jones and Anna Chen and Anna Goldie and Azalia Mirhoseini and Cameron McKinnon and Carol Chen and Catherine Olsson and Christopher Olah and Danny Hernandez and Dawn Drain and Deep Ganguli and Dustin Li and Eli Tran-Johnson and Ethan Perez and Jamie Kerr and Jared Mueller and Jeffrey Ladish and Joshua Landau and Kamal Ndousse and Kamile Lukosuite and Liane Lovitt and Michael Sellitto and Nelson Elhage and Nicholas Schiefer and Noemi Mercado and Nova DasSarma and Robert Lasenby and Robin Larson and Sam Ringer and Scott Johnston and Shauna Kravec and Sheer El Showk and Stanislav Fort and Tamera Lanham and Timothy Telleen-Lawton and Tom Conerly and Tom Henighan and Tristan Hume and Samuel R. Bowman and Zac Hatfield-Dodds and Ben Mann and Dario Amodei and Nicholas Joseph and Sam McCandlish and Tom Brown and Jared Kaplan},
      year={2022},
      eprint={2212.08073},
      archivePrefix={arXiv},
      primaryClass={cs.CL}
}

\begin{figure}[t]
    \centering
    \includegraphics[width=\linewidth]{image/target.png}
    % \vspace{-0.2in}
    \caption{By adding noise (e.g., shuffling, deletion) to the human written reference (gold reference) and substitution on original sentences, we can acquire adversarial examples with different characteristics: high adequacy, low simplicity, or vice versa.}
    \label{fig:target}
    %\vskip -1em
    % \vspace{-0.2in}
\end{figure}

\subsection{Annotation Quality}
\begin{table}[t]
% \small
% \footnotesize
\scriptsize
    \centering
    \begin{tabular}{p{1.0cm}|p{1.15cm}<{\centering}|p{1.15cm}<{\centering}|p{1.15cm}<{\centering}|p{1.15cm}<{\centering}}
    % \begin{tabular}{c|c|c}
    \toprule
        Model & G & M & S & StS  \\
         \midrule
        Overall & 0.70(0.63) & 0.63(0.75) & 0.77(0.41) & 0.65(0.27) \\
        \midrule
        % \hline
        Reference & 0.81(0.24) & 0.73(0.59) & 0.61(0.49) & 0.57(0.48) \\
        \midrule
        Dress & 0.91(0.58) & 0.74(0.86) & 0.86(0.28) & 0.54(0.26) \\
        Hybrid & 0.46(0.58) & 0.53(0.68) & 0.93(0.27) & 0.29(-0.05) \\
        PBMT & 0.77(0.53) & 0.61(0.55) & 0.66(0.44) & 0.74(0.30) \\
        \midrule
        % \hline
        UNTS & 0.63(0.69) & 0.61(0.79) & 0.79(0.22) & 0.74(0.12)  \\
        % \hline
        EditUTS & 0.60(0.47) & 0.50(0.42) & 0.71(0.18) & 0.71(0.33)  \\

        BRTLTS & 0.69(0.34) & 0.63(0.70) & 0.77(0.32) & 0.84(0.42) \\
        BTTS10 & 0.76(0.74) & 0.64(0.88) & 0.84(0.49) & 0.77(0.36) \\
        
         \bottomrule
    \end{tabular}
    \caption{Average pairwise absolute agreement and Cohen's quadratic weighted kappa (in bracket) for annotators for the systems on four aspects described in Section~\ref{sec:exp-setup}. BTTS10 indicates the semi-supervised BTTS model with 10\% training data. }%We use the ``RM+EX+LS+RO'' variant for the EditUTS model.}
    \label{tab:annotation-IAA}
    %\vspace{-0.2in}
\end{table}

 Table~\ref{tab:annotation-IAA} presents the scores for system quality annotation. The overall agreement with all systems and metrics is 0.69 (for pairwise absolute agreement) and 0.94 (for quadratic weighted kappa). Such good agreement for a question with 5 options shows that the annotators can understand and solve the tasks well. The quality of the agreement and comparatively lower agreement on evaluating simplicity (i.e., S and StS) also match the annotation results from previous work \cite{sulem-etal-2018-semantic}.
